# Supplementary material for: ReChorus2.0: A Modular and Task-Flexible Recommendation Library
Source: arXiv:2405.18058 source file (2024-05-28)
Supplement: Supplementary file 1 [file appendix.tex]

%%
%% If your work has an appendix, this is the place to put it.
\appendix
